# Supplementary material for: Correlation effects on ground-state properties of ternary Heusler alloys: first-principles study
Source: arXiv:1901.09460 ancillary file (2019-01-27)
Supplement: Supplementary file 1 [file SupplementaryPRB2018.pdf]

# Supplementary material for "Correlation effects on ground-state properties of ternary Heusler alloys: first-principles study"

V.D. Buchelnikov[1,2], V.V. Sokolovskiy[1,2], O.N. Miroshkina[1], M.A. Zagrebin[1,2,3], J. Nokelainen[4], A. Pulkkinen[4], B. Barbiellini[4,5], and E. Lähderanta[4]
[1]*Faculty of Physics, Chelyabinsk State University, 454001 Chelyabinsk, Russia*
[2]*National University of Science and Technology "MISiS", 119049 Moscow, Russia*
[3]*National Research South Ural State University, 454080 Chelyabinsk, Russia*
[4]*Lappeenranta University of Technology, FI-53851 Lappeenranta, Finland and*
[5]*Department of Physics, Northeastern University, Boston, MA 02115, USA*

In order to provide deeper analysis of the SCAN functional, we performed additional calculations for half-metallic $Co_2FeSi$ and semiconductor CoFeTiAl Heusler compounds, for which the correlation effects are expected to play a prevailing role in electronic structure. Electronic structure calculations with PBE and SCAN functionals were performed using 8-atom cubic supercell for $Co_2FeSi$ and CoFeTiAl with the space group of $Fm\bar{3}m$ and $F\bar{4}3m$, respectively. For the latter structure, Co, Fe, Ti, and Al occupy $4c$ (1/4, 1/4, 1/4), $4d$ (3/4, 3/4, 3/4), $4b$ (1/2,1/2,1/2), and $4a$ (0, 0, 0) positions, correspondingly. Ferromagnetic ordering was considered for both compositions.

Fig. S**??** presents calculated total energy differences as a function of lattice constant for $Co_2FeSi$ and CoFeTiAl. It is seen from this figure that equilibrium lattice parameter calculated with SCAN is less than calculated with PBE one. This difference is about 1% for both compounds. PBE lattice parameter is closer to experimental value with respect to SCAN one (see Table S**??**).

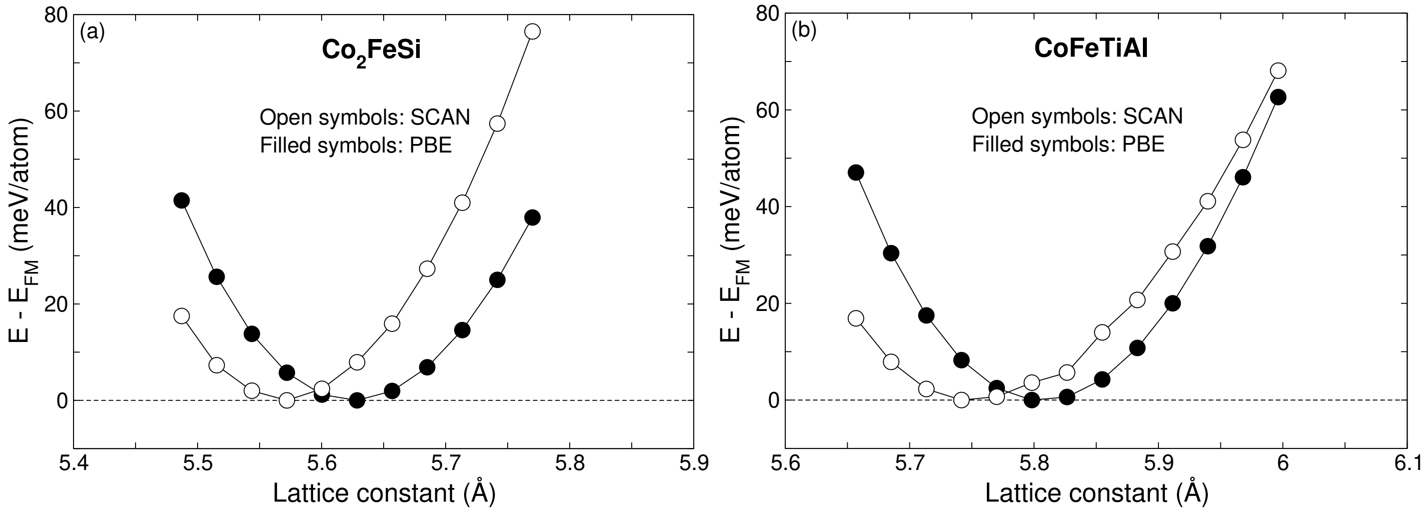


FIG. S 1: (Colour online) The total energy differences as a function of lattice constant for cubic (a) $Co_2FeSi$ and (b) CoFeTiAl calculated with PBE and SCAN.

The dependencies of energy difference on the tetragonal distortion $c/a$ for $Co_2FeSi$ and CoFeTiAl are shown in Fig. S**??**. For $Co_2FeSi$, PBE calculations yield the tendency to pseudomartensitic transformation. This trend is associated with evident minimum of $\Delta E\,(c/a)$ function with $c/a > 1$. However, the energy of the pseudotetragonal distorted phase ($c/a > 1$) is higher than the cubic one. On the contrary to PBE, SCAN results do not give a tendency to pseudomartensitic transition, and $\Delta E\,(c/a)$ curve has the one minimum corresponding to the cubic phase ($c/a = 1$). In case of CoFeTiAl, energy curves have just one minimum at $c/a = 1$ and demonstrate the similar behavior for both PBE and SCAN.

Electronic densities of states (DOS) for $Co_2FeSi$ and CoFeTiAl calculated at the optimized lattice parameter with the help of PBE and SCAN are presented in Fig. S**??**. For $Co_2FeSi$, it is seen that calculated DOS for the majority spin band have the metallic nature due to occupied band at the Fermi level ($E_F$). As for minority spin band, PBE yields the pseudo half-metallic behavior due to presence of the energy gap shifted slightly to lower energies with respect to $E_F$. However, SCAN DOS for the minority spin reveals the energy gap near $E_F$ which indicates the half-metallic behavior. For CoFeTiAl nonmagnetic semiconductor behavior results from both PBE and SCAN DOSs curves. Besides, the value of SCAN energy gap is slightly higher than PBE one.

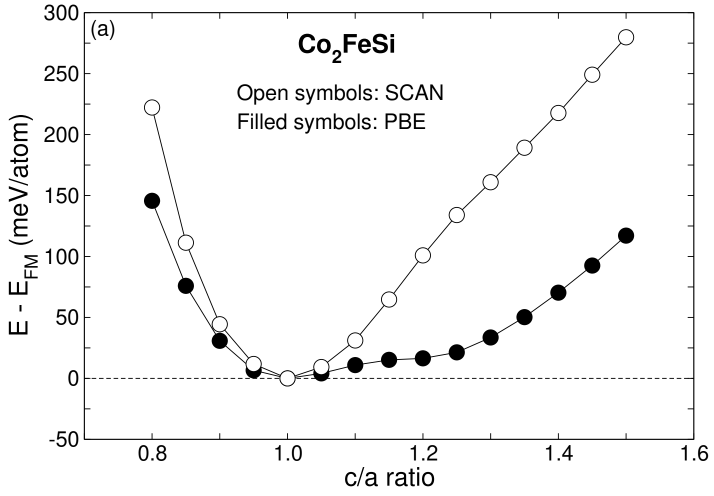


FIG. S 2: (Colour online) The calculated total energy differences as a function of tetragonal ratio $c/a$ for (a) Co2FeSi and (b) CoFeTiAl.

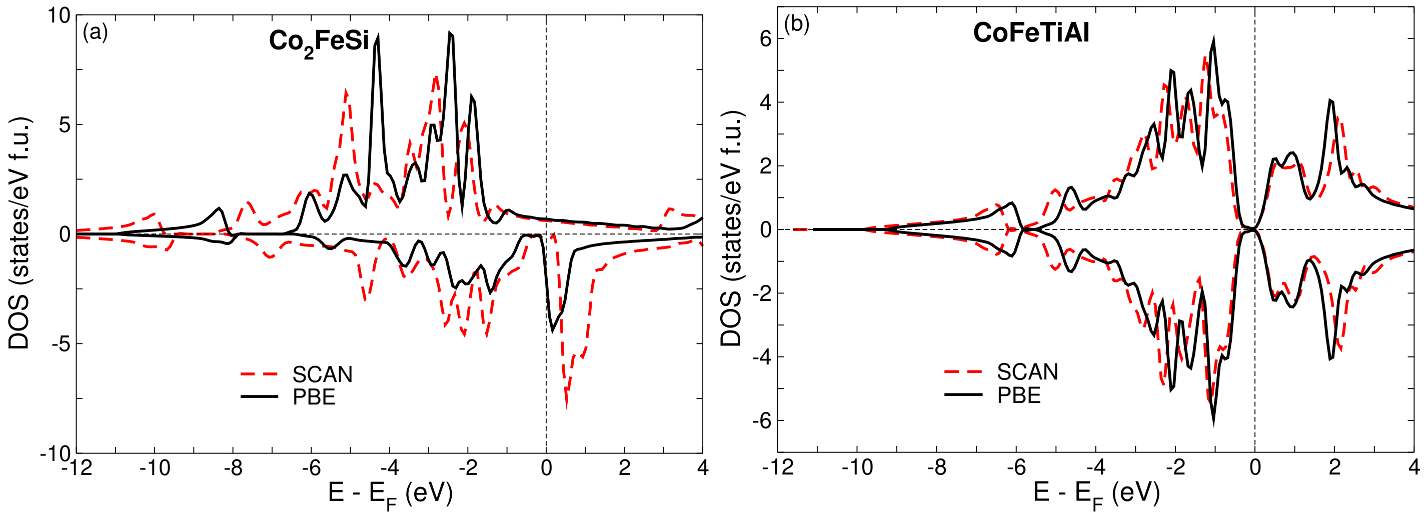


FIG. S 3: (Colour online) The total DOS calculated with PBE and SCAN for the austenitic phase of (a) $Co_2FeSi$ and (b) CoFeTiAl Heusler compounds. Here the solid and dash lines denote the PBE and SCAN calculations.

The equilibrium lattice constants $a_0$ and total magnetic moments $\mu$ calculated with the help of PBE and SCAN are summarized in Table S??. SCAN total magnetic moments for $Co_2FeSi$ and CoFeTiAl are nearly integer and satisfy the Slater-Pauling rule ($\mu_{tot} = N_V - 24$), where $N_V$ is the number of valence electrons in the unit cell consisting of four atoms. In general, for both $Co_2FeSi$ and CoFeTiAl, the results of SCAN calculations are in good agreement with the ones of GW approximation[?] [?] .

TABLE S I: The equilibrium lattice constants $a_0$ and total magnetic moments $\mu$ calculated with PBE and SCAN in comparison with the available experimental data. $N_V$ is the number of valence electrons.

| | $N_V$ | $a_0$ [Å] | | | Magnetic moment [$\mu_B$/f.u.] | | |
|---|---|---|---|---|---|---|---|
| | | PBE | SCAN | exp. | PBE | SCAN | exp. |
| $Co_2FeSi$ | 30 | 5.625 | 5.570 | 5.64 [?] | 5.534 | 6.022 | 5.65 [?] |
| CoFeTiAl | 24 | 5.806 | 5.756 | 5.851 | 0 | 0 | 0 [?] |

[1] M. Meinert, Ch. Friedrich, G.Reiss, S. Blügel, Phys. Rev. B **86**, 245115 (2012).
[2] M. Tas, E. Şaşıoğlu, I. Galanakis, C. Friedrich, S. Blügel, Phys. Rev. B **93**, 195155 (2016).
[3] B. Balke, S. Wurmehl, G. H. Fecher, C. Felser, M.C.M. Alves, F. Bernardi, J. Morais, Appl. Phys. Lett. **90**, 172501 (2007).
[4] B. Deka, D. Chakraborty, A. Srinivasan, Physica B **448**, 173 (2014).
[5] *Spintronics: from Materials to Devices* ed by C. Felser and G.H. Fecher (New York: Springer) p 369 (2013).
